# Supplementary material for: The curious case of developmental BERTology: On sparsity, transfer learning, generalization and the brain
Source: arXiv:2007.03774 source file (2020-07-07)
Supplement: Supplementary file 1 [file supplement.tex]

\section{Problem statement}

\begin{table*}[t]
\caption{Fine-tuning by sparsification}
\begin{center}
\begin{small}
\begin{tabular}{l | c c c c c c c}
    \toprule
    \begin{tabular}{@{}l@{}}
        \multirow{2}{*}{
            \begin{tabular}{@{}l@{}}Model\end{tabular}
        }
    \end{tabular} & 
    \multicolumn{6}{c}{Fine-tune structure on mixture $\lambda \bm\theta^\text{random} + (1-\lambda) \bm\theta^\text{pre-trained}$} \\
    &
    \begin{tabular}{@{}l@{}}
        $\lambda = 0$ 
    \end{tabular} & 
    \begin{tabular}{@{}l@{}}
        $\lambda = 2^{-5}$ 
    \end{tabular} & 
    \begin{tabular}{@{}l@{}}
        $\lambda = 2^{-4}$ 
    \end{tabular} & 
    \begin{tabular}{@{}l@{}}
        $\lambda = 2^{-3}$ 
    \end{tabular} & 
    \begin{tabular}{@{}l@{}}
        $\lambda = 2^{-2}$ 
    \end{tabular} & 
    \begin{tabular}{@{}l@{}}
        $\lambda = 2^{-1}$ 
    \end{tabular} & 
    \begin{tabular}{@{}l@{}}
        $\lambda = 1$ 
    \end{tabular} \\
    \midrule
    \texttt{bert-base} & 
        \bf .9035 $\pm$ .0032 & \bf .8953 $\pm$ .0038 & \bf .9037 $\pm$ .0074 & \bf .9015 $\pm$ .0075 & .8382 $\pm$ .0092 & - & .7937 $\pm$ .0079 \\
    \texttt{bert-large} & 
        \bf .8996 $\pm$ .0020 & \bf .9021 $\pm$ .0060 & \bf .9057 $\pm$ .0077 & \bf .9114 $\pm$ .0022 & .8675 $\pm$ .0122 & - & .8122 $\pm$ .0000 \\
    \midrule
    \texttt{xlnet-base} & 
        \bf .9061 $\pm$ .0048 & - & \bf .9016 $\pm$ .0085 & \bf .8960 $\pm$ .0120 & \bf .9032 $\pm$ .0091 & .8612 $\pm$ .0112 & .8122 $\pm$ .0000 \\
    \texttt{xlnet-large} & 
        \bf .9048 $\pm$ .0038 & - &     .8681 $\pm$ .0484 & \bf .9009 $\pm$ .0124 &     .8735 $\pm$ .0445 & .8250 $\pm$ .0117 & .8122 $\pm$ .0000 \\
    \midrule
    \texttt{roberta-base} & 
        \bf .9031 $\pm$ .0025  & - & \bf .9108 $\pm$ .0027 &     .8885 $\pm$ .0032 & .8292 $\pm$ .0108 & .8085 $\pm$ .0058 & .8029 $\pm$ .0084 \\
    \texttt{roberta-large} & 
        \bf .9186 $\pm$ .0066  & - & \bf .9102 $\pm$ .0038 & \bf .9034 $\pm$ .0083 & .8062 $\pm$ .0105 & .7817 $\pm$ .0219 & .7846 $\pm$ .0171 \\
    \midrule
    \texttt{albert-base} & 
        \bf .8984 $\pm$ .0064 & - & \bf .9005 $\pm$ .0078 &     .8761 $\pm$ .0061 & .8050 $\pm$ .0092 & .8008 $\pm$ .0134 & .7893 $\pm$ .0070 \\
    \texttt{albert-large} & 
        \bf .9080 $\pm$ .0029 & - & \bf .9071 $\pm$ .0075 & \bf .8949 $\pm$ .0126 & .8056 $\pm$ .0073 & .7954 $\pm$ .0077 & .7898 $\pm$ .0080 \\
    \texttt{albert-xlarge} & 
        \bf .9096 $\pm$ .0062 & - & \bf .9093 $\pm$ .0019 & \bf .9069 $\pm$ .0032 & .7885 $\pm$ .0357 & .7768 $\pm$ .0111 & - \\
    \bottomrule
\end{tabular}
\end{small}
\end{center}
\vskip -0.1in
\end{table*}

\begin{table*}[t]
\caption{Fine-tuning}
\begin{center}
\begin{small}
\begin{tabular}{l | c c c c c c c}
    \toprule
    \begin{tabular}{@{}l@{}}
        \multirow{2}{*}{
            \begin{tabular}{@{}l@{}}Model\end{tabular}
        }
    \end{tabular} & 
    \multicolumn{6}{c}{Fine-tune weights from mixture $\lambda \bm\theta^\text{random} + (1-\lambda) \bm\theta^\text{pre-trained}$} \\
    &
    \begin{tabular}{@{}l@{}}
        $\lambda = 0$ 
    \end{tabular} & 
    \begin{tabular}{@{}l@{}}
        $\lambda = 2^{-5}$ 
    \end{tabular} & 
    \begin{tabular}{@{}l@{}}
        $\lambda = 2^{-4}$ 
    \end{tabular} & 
    \begin{tabular}{@{}l@{}}
        $\lambda = 2^{-3}$ 
    \end{tabular} & 
    \begin{tabular}{@{}l@{}}
        $\lambda = 2^{-2}$ 
    \end{tabular} & 
    \begin{tabular}{@{}l@{}}
        $\lambda = 2^{-1}$ 
    \end{tabular} & 
    \begin{tabular}{@{}l@{}}
        $\lambda = 1$ 
    \end{tabular} \\
    \midrule
    \texttt{bert-base} & 
        \bf .8890 $\pm$ .0061 & \bf .8913 $\pm$ .0106 & \bf .8970 $\pm$ .0132 & \bf .8942 $\pm$ .0013 & .8378 $\pm$ .0144 & - & .7754 $\pm$ .0134 \\
    \texttt{bert-large} & 
        \bf .8968 $\pm$ .0148 & \bf .8975 $\pm$ .0155 & \bf .9020 $\pm$ .0111 & \bf .9054 $\pm$ .0060 & .8305 $\pm$ .0411 & - & .8122 $\pm$ .0000 \\
    \midrule
    \texttt{xlnet-base} & 
        \bf .8950 $\pm$ .0159 & - & \bf .8938 $\pm$ .0096 & \bf .8977 $\pm$ .0027 & \bf .8960 $\pm$ .0122 & .8482 $\pm$ .0033 & .7897 $\pm$ .0212 \\
    \texttt{xlnet-large} & 
        \bf .9132 $\pm$ .0051 & - &     .8696 $\pm$ .0497 & \bf .9119 $\pm$ .0040 & \bf .9047 $\pm$ .0020 & .8086 $\pm$ .0063 & .8122 $\pm$ .0000 \\
    \midrule
    \texttt{roberta-base} & 
        \bf .9131 $\pm$ .0057  & - & \bf .9164 $\pm$ .0058 & \bf .9201 $\pm$ .0033 & .8198 $\pm$ .0027 & .8005 $\pm$ .0133 & .7972 $\pm$ .0097 \\
    \texttt{roberta-large} & 
        \bf .9158 $\pm$ .0028  & - & \bf .9159 $\pm$ .0081 & \bf .9025 $\pm$ .0120 & .8087 $\pm$ .0082 & .8065 $\pm$ .0100 & .8122 $\pm$ .0000 \\
    \midrule
    \texttt{albert-base} & 
        \bf .9008 $\pm$ .0056 & - & \bf .8967 $\pm$ .0034 & \bf .8843 $\pm$ .0141 & .8011 $\pm$ .0157 & .7939 $\pm$ .0102 & .7816 $\pm$ .0105 \\
    \texttt{albert-large} & 
        \bf .9108 $\pm$ .0021 & - & \bf .9063 $\pm$ .0039 & \bf .8981 $\pm$ .0116 & .8008 $\pm$ .0151 & .8122 $\pm$ .0000 & .8041 $\pm$ .0141 \\
    \texttt{albert-xlarge} & 
        \bf .9043 $\pm$ .0025 & - & \bf .9074 $\pm$ .0077 & \bf .9050 $\pm$ .0027 & .7872 $\pm$ .0030 & .7769 $\pm$ .0148 & .7805 $\pm$ .0550 \\
    \bottomrule
\end{tabular}
\end{small}
\end{center}
\vskip -0.1in
\end{table*}
